# Supplementary material for: LES of a classical hydraulic jump: Influence of modelling parameters on the predictive accuracy
Source: arXiv:2007.01729 source file (2020-07-03)
Supplement: Supplementary file 1 [file appendicies.tex]

\section{The influence of spanwise domain length} \label{app:spanwise}

\section{The influence of surface tension} \label{app:surface_tension}

\section{Higher CFL number simulations} \label{app:cfl}
